# Supplementary material for: A Maturity Assessment Framework for Conversational AI Development Platforms
Source: arXiv:2012.11976 source file (2020-12-22)
Supplement: Supplementary file 1 [file Supplementary.pdf]

Table 1: Search strings used to find start set for snowballing.

| | |
|---|---|
| 1 | Conversational AI |
| 2 | Chatbots |
| 3 | Chatbot language |
| 4 | Chatbot feature |
| 5 | Conversational AI language |
| 6 | Conversational AI systems |
| 7 | Conversational AI features |
| 8 | Conversational AI development |
| 9 | Conversational AI comprehension |
| 10 | Chatbot comprehension |
| 11 | Developing AI chatbots |
| 12 | Conversational Agents |
| 13 | Conversational platforms |
| 14 | Conversational AI platforms |
| 15 | Conversational AI development platforms |
| 16 | Chatbot development |
| 17 | Chatbot platforms |
| 18 | Conversational AI comparison |
| 19 | Conversational Agent development platforms |
| 20 | Dialog management |
| 21 | Dialog management in chatbots |
| 22 | Dialog management conversational AI |
| 23 | Mandatory chatbot features |
| 24 | Common chatbot features |
| 25 | Conversational AI characteristics |
| 26 | Chatbot characteristics |
| 27 | Mandatory conversational AI features |
| 28 | Dialog flow development |
| 29 | IBM watson development |
| 30 | Amazon lex development |
| 31 | Microsoft bot framework development |
| 32 | VoiceXML |
| 33 | VoiceXML conversational AI |

Table 2: Search strings used to find systems for the analysis.

| | |
|---|---|
| 1 | Alternatives to *platform* |
| 2 | *platform* competitors |
| 3 | *platform* alternatives |
| 4 | Systems similar to *platform* |
| 5 | Systems like *platform* |
| 6 | *platform* like systems |
| 7 | Platforms like *platform* |
| 8 | Platforms similar to *platform* |
| 9 | Applications similar to *platform* |
| 10 | Applications like *platform* |
| 11 | *platform* like applications |

Table 3: Search strings used for literature review for creation of conversational maturity framework.

| | |
|---|---|
| 1 | Common language framework |
| 2 | Human language framework |
| 3 | Language framework |
| 4 | Developing language framework |
| 5 | developing conversational AI language framework |
| 6 | Understanding language frameworks |
| 7 | Conversational AI language framework |
| 8 | Conversational AI language evaluation |
| 9 | Conversational AI understanding language |
| 10 | Conversational AI language levels |
| 11 | Conversational AI language comprehension |
| 12 | Natural language framework |
| 13 | Natural Language Evaluation |
| 14 | Natural Language Complexity |
| 15 | Natural Language Comprehension |
| 16 | Conversational AI Language Maturity |
| 17 | Conversational AI Maturity |

Table 4: List of papers used as start set for snowballing and which systems were found.

| **Paper** | **Systems found** |
|---|---|
| T. Bocklisch, J. Faulkner, N. Pawlowski, and A. Nichol, "Rasa: Open Source Language Understanding and Dialogue Management", tech. rep., NIPS 2017 Conversational AI workshop, Long Beach, 2017 | RASA |

| Continuation of Table 4 | |
|---|---|
| Paper | Systems found |
| R. I. A. Bohus, Dan, "The RavenClaw dialog management framework: Architecture and systems", Computer Speech & Language, vol. 23, pp. 332–361, 2009. | VoiceXML, RavenClaw |
| J. Rouillard, "Web services and speech-based applications around VoiceXML", tech. rep., Université des Sciences et Technologies de Lille, Villeneuve d'Ascq Cedex, 2006 | VoiceXML |
| P. Milhorat, S. Schlögl, G. Chollet, J. Boudy, A. Esposito, and G. Pelosi, "Building the next generation of personal digital assistants", ATSIP 2014: 1st International Conference on Advanced Technologies for Signal and Image Processing, pp. 458–463, 2014. | Siri, Amazon Alexa, Google Assistant |
| M. Mctear, "Conversational modelling for chatbots: current approaches and future directions", tech. rep., Ulster University, 2018 | DialogFlow, Amazon Lex, Microsoft Bot Framework, IBM Watson Conversation |
| P. Priya Angara, Towards a Deeper Understanding of Current Conversational Frameworks through the Design and Development of a Cognitive Agent. PhD thesis, Gandhi Institute of Technology and Management, 2018. | DialogFlow, Amazon Lex, Microsoft Bot Framework, IBM Watson Conversation, Wit.ai, RASA |
| R. Sarikaya, P. A. Crook, A. Marin, M. Jeong, J. P. Robichaud, A. Celikyilmaz,Y. B. Kim, A. Rochette, O. Z. Khan, X. Liu, D. Boies, T. Anastasakos, Z. Feizol-lahi, N. Ramesh, H. Suzuki, R. Holenstein, E. Krawczyk, and V. Radostev, "An overview of end-to-end language understanding and dialog management for personal digital assistants", tech. rep., Microsoft Corporation, Redmond, WA, 2016 | Cortana |
| M. Mctear, Z. Callejas, and D. Griol, The Conversational Interface Talking to Smart Devices. Springer International Publishing, 2016 | Amazon Lex, Microsoft LUIS, VoiceXML, API.ai, AIML, wit.ai, IBM Watson Conversation, TrindiKit/ Dipper, NextIt, Interactions and Nuance nina |

| Continuation of Table 4 | |
|---|---|
| Paper | Systems found |
| C. Massimo and L. De Russis, "A Comparison and Critique of Natural Language Understanding Tools", in Cloud computing 2018 (B. Duncan, Y. Woo Lee,and A. Olmsted, eds.), (Barcelona), pp. 110–115, Researchgate, 2018 | wit.ai, LUIS, IBM Watson Conversation, Amazon Lex, Recast.ai |
| J. Gao, M. Galley, L. Li, G. Brain, C. Brockett, A. Celikyilmaz, Y. Cheng,B. Dolan, P. Fung, Z. Gan, S. Lee, J. Li, X. Li, B. Liu, A. Madotto, R. Ma-jumder, A. Papangelis, O. Pietquin, C. Quirk, A. Ritter, P. Smolensky, A. Sor-doni, Y. Song, H. Suzuki, W. Wei, T. Weiss, K. Yuan, and Y. Zhang, "Neural Approaches to Conversational AI Question Answering, Task-Oriented Dialogues and Social Chatbots", tech. rep., 2018 | LUIS, DialogFlow, Amazon Lex, IBM Watson Conversation, Cortana, Alexa, XiaoIce, Replika, Zo, Ruuh, Bing QA, Satori QA |

Table 5: List of papers found in first iteration of snowballing.

| Paper | Systems found |
|---|---|
| D. Braun, A. Hernandez Mendez, F. Matthes, and M. Langen, "Evaluating Natural Language Understanding Services for Conversational Question Answering Systems", in Proceedings of the SIGDIAL 2017 Conference, (Saarbrucken), pp. 174–185, Association for Computational Linguistics, 2017 | IBM Watson, wit.ai, Amazon Lex |
| R. Kar and R. Haldar, "Applying Chatbots to the Internet of Things: Opportunities and Architectural Elements", tech. rep., School of Computing Sciences and Engineering, VIT University, Vellore, India, 2016 | wit.ai, Microsoft Bot Framework |
| M. F. Mctear, "Spoken Dialogue Technology: Enabling the Conversational User Interface", tech. rep., University of Ulster, Ulster, 2002 | VoiceXML, CPK Generic Dialogue System Platform, CSLU toolkit, CU Communicator system, GULAN, IBM voice server, NLSA, NUANCE, Speech Mania, Vocalis SpeechWare |
| J. Rouillard and P. Truillet, "Enhanced VoiceXML", tech. rep., 2005 | VoiceXML |
| R. Catizone, A. Setzer, and Y. Wilks, "State of the Art in Dialogue Management", tech. rep., 2002 | TrindiKit, SUN-Dial |
| D. Bohus and A. I. Rudnicky, "RavenClaw: Dialog Management Using Hierarchical Task Decomposition and an Expectation Agenda", tech. rep., Carnegie Mellon University, Computer Science Department, Pittsburgh, PA, 2003 | TeamTalk, BusLine, RoomLine, LARRI, RavenClaw |
| S. Larsson, "User-initiated Sub-dialogues in State-of-the-art Dialogue Systems", in Proceedings of the SIGDIAL 2017 Conference, (Saarbrücken, Germany), pp. 17–22, Department of Philosophy, Linguistics and Theory of Science University of Gothenburg, Association for Computational Linguistics, 2017 | Siri, API.AI, Houndify, Cortana, Alexa |
| E. Fast, B. Chen, J. Mendelsohn, J. Bassen, and M. Bernstein, "Iris: A Conversational Agent for Complex Tasks", tech. rep., Stanford University, 2017 | Iris |

| Continuation of Table 5 | |
|---|---|
| Paper | Systems found |
| L. Cuno Klopfenstein, S. Delpriori, S. Malatini, and A. Bogliolo, "The Rise of Bots: A Survey of Conversational Interfaces, Patterns, and Paradigms", tech.rep., Department of Pure and Applied Sciences, Urbino, Italy, 2017 | AIML, ALICE, Alexa, Google assistant, Cortana, Samsung S voice, Anna by IKEA, CHARLIE, MOOCBuddy, Nombot, SUNDIAL |
| L. Wanner, E. André, J. Blat, S. Dasiopoulou, M. Farrùs, T. Fraga, E. Kamateri,F. Lingenfelser, G. Llorach, O. Martínez, G. Meditskos, S. Mille, W. Minker,L. Pragst, D. Schiller, A. Stam, L. Stellingwerff, F. Sukno, B. Vieru, and S. Vrochidis, "KRISTINA: A Knowledge-Based Virtual Conversation Agent", in Advances in Practical Applications of Cyber-Physical Multi-Agent Systems: The PAAMS Collection (Y. Demazeau, P. Davidsson, J. Bajo, and Z. Vale, eds.), pp. 284–295, Springer, Cham, 2017 | KRISTINA |
| P. A. Crook, A. Marin, V. Agarwal, K. Aggarwal, T. Anastasakos, R. Bikkula,D. Boies, A. Celikyilmaz, S. Chandramohan, Z. Feizollahi, R. Holenstein,M. Jeong, O. Z. Khan, Y.-B. Kim, E. Krawczyk, X. Liu, D. Panic, V. Radostev,N. Ramesh, J.-P. Robichaud, A. Rochette, L. Stromberg, and R. Sarikaya, "Task Completion Platform: A self-serve multi-domain goal oriented dialogue platform", in Proceedings of NAACL-HLT 2016 (Demonstrations), (San Diego, CA), pp. 47–51, Association for Computational Linguistics, 2016 | VoiceXML, RavenClaw, ClippyScript, TCP |
| G. De Gasperis, I. Chiari, and N. Florio, "AIML Knowledge Base Construction from Text Corpora", in Artificial Intelligence, Evolutionar Computing and Metaheuristics (Janusz Kacprzyk and Xin She Yang, eds.), pp. 287–318, Springer, Berlin, Heidelberg, 2013 | AIML |
| A. Patil, M. K, N. R. A, and N. R, "Comparative study of cloud platforms to develop a Chatbot,"International Journal of Engineering & Technology, vol. 6, p. 57, 6 2017 | IBM Watson Conversation, chatfuel, Heroku, Kore, Amazon Lex |

Table 6: List of papers found in second iteration of snowballing.

| Paper | Systems found |
|---|---|
| F. Morbini, K. Audhkhasi, K. Sagae, R. Artstein, D. Gan Can, P. Georgiou,S. Narayanan, A. Leuski, and D. Traum, "Which ASR should I choose for my dialogue system?", in Proceedings of the SIGDIAL 2013 Conference, (Metz), p. 394–403, Association for Computational Linguistics, 2013 | DialogFlow, Siri, AT&T Watson |
| B. A. Shawar and E. Atwell, "Different measurements metrics to evaluate a chat-bot system", in Bridging the Gap: Academic and Industrial Research in Dialog Technologies Workshop Proceedings, (Rochester, NY), pp. 89–96, Association for Computational Linguistics, 2007 | AIML |
| G. Campagna, R. Ramesh, S. Xu, M. Fischer, and M. S. Lam, "Almond: The Architecture of an Open, Crowdsourced, Privacy-Preserving, Programmable Virtual Assistant", in Proceedings of the 26th International Conference on World Wide Web - WWW '17, (New York, New York, USA), pp. 341–350, ACM Press,2017 | Almond |

Table 7: List of feature descriptions. Written in bold is features that have underlying features and written in italics is abstract features. The features are in order of the feature model.

| **Feature name** | **Description** |
|---|---|
| ***System*** | Features regarding the system and the supported tools and platforms. |
| ***Content*** | Features regarding the content of conversations that a system offers. A content of a conversation is i.e. "Booking" or " Setting an alarm". |
| ContentCatalogs | The system has in-built content catalogues to simplify the development of the conversational AI bot. These catalogs contain entities and intents that are common within the selected field. |
| MultipleConversation-Domains | The system is built with domains that is independent from one another. Thus making the system support multiple domains under one conversation. |
| ***Development*** | Features regarding the development process of the conversational AI systems. |
| ErrorFeedback | The system provides error messages upon a error occuring, which is used to give the developer some feedback on what went wrong in the system. |
| MultiProgramming-Language | The system has support for two or more programming languages. |

| Continuation of Table 7 | |
|---|---|
| **Feature name** | **Description** |
| PredefinedSlotTypes | The system has in-built slot types that are common in conversations. Typical examples for built-in slot types include e-mail adresses, phone numbers and ZIP codes. |
| SystemVersioning | The system supports iterative development of the system with versioning. |
| **TrainingData** | The system uses training data to generate a NLU model for the conversational AI system. This model is used for NLP in the system to understand the input. |
| CustomTrainingData | The system allows for the developer to choose what data set the developers wants to use for training the NLU model. |
| ***ProgrammingTools*** | The system has in-built tools to help developers by simplifying the development process. |
| DebugTool | Debug tools that are available within the system development that are readily available for the developers to use. |
| ModelEvaluation | Lets the developer evaluate the NLU model generated by the system, for analysis purposes such as: to see if it fits the companies purpose. |
| VisualisationTools | Tools to simplify for the developer using visual aids, these can vary from visualising the dialog tree to drag and drop boxes for entities and intents. |
| **InputProcessing** | Features regarding the processing of the user inputs. |
| AutomaticUnderstanding | The conversation is automatically processed using Natural Language Understanding to get the system to understand what the user says and writes. |
| MultiLanguage | The system has support for two or more languages. |
| Propositionality | Distinguishes semantic roles for different answers of same sort, e.g. "from X to Y" vs "to X from Y". |
| SpellingCorrection | The system automatically corrects spelling mistakes to make it easier for it to understand what the user means. This has a threshold on how much it can auto correct just like typing on a phone. |
| ***LanguageRecognition*** | The system can automatically detect the language which the user is inputing. I.e. "Hola como te llamas?" will be detected as input in spanish. |
| Translation | The system can translate conversations to any supported language. This requires the system to have LanguageRecognition. |
| ***Interfaces*** | Features regarding the different interfaces supported by the system. |
| FrontendIntegration | The system allows for calls to be made to the frontend interface, i.e. make phonecalls or send text messages via the phone. |

| Continuation of Table 7 | |
|---|---|
| **Feature name** | **Description** |
| SocialPlatformSupport | The system is integratable with social platforms such as Facebook, Slack or Instagram. This allows the developer to create chatbots within the platforms directly. |
| WebIntegration | The system allows for webhooks and other calls to the web, i.e. google searches and pulling weather information from the web. |
| | |
| ***Conversation*** | Features regarding the conversational part of the system. |
| LanguageSeparation | The system can separate between language-specific and non-language-specific information, to simplify translation and multi language maintenance. |
| ***ConversationOutput*** | Features regarding the system outputs during conversations. |
| DialogInitiation | The system allows for the developer to set if the bot shall initiate conversation or if it shall wait for the user to initialise. |
| Policies | Policies are used for dialogs and conversation, to set restrictions and guidelines. These can be anything from restricted words to censorship. |
| Sentiments | Sentiments are similar to human emotions such as angry, sad and happy. The system allows for the developer to set a overall system sentiment. |
| **Clarification** | Features regarding clarification of the users input, to let the system know that the information received is not incorrect. |
| Affirmation | Affirmation is used by the system to confirm the intent of the user. Examples: (User) What is the weather like in Göteborg? (Bot) Did you ask for the weather in Göteborg? |
| FallbackActions | Fallback actions is a mechanism used by the system if it didn't understand what the user said/wrote. These actions can be something like: (Bot) I didn't understand, please try again. |
| Rephrasing | Rephrasing is used by the system to confirm the intent of the user. Examples: (Bot) Did you mean Gothenburg? |
| ***ConversationTypes*** | Different conversation types that the system has support for. |
| SearchOrientedDialog | The system organizes different slot types in groups to simplify searches and to be able to quantify how many hits the system got from a specific search. I.e. (User) Search for Johan. (Bot) There where 12 Johan's found. |
| SlotFilling | The system will ask follow up questions to statements that are missing information, for example: (User) What is the weather like today? (Bot) Where would you like to check the weather for? |

| Continuation of Table 7 | |
|---|---|
| **Feature name** | **Description** |
| **ContextualDialogs** | The possibility to hold more complex dialogs that keep the context throughout the conversation, The system will remember what the user has said/written previously. |
| MemoryForContext | The system keeps conversation history to keep the context of the conversation, this memory size can vary depending on system. |
| TopicShifting | The system allows for multi-contextual dialogs, a dialog where the user switches between contexts. Allowing the user to converse about the weather whilst also conversing about the upcoming events in the area. |
| ***Questions*** | Features regarding the question part of the conversations. |
| MultipleUserIntents | The system allows for phrases/ sentences with multiple questions, usually supports no more than 3 questions in one phrase. |
| **OneShotQueries** | A user command that only requires an answer with no further conversation needed. I.e. (User) Tell me the time. (Bot) The time is 12:43. |
| OpenQuestion | The system supports for the use of open questions. Examples "What is the weather like?" & "How far is it to Stockholm?" |
| YesNoQuestion | The system supports questions that only require a yes or no answer from the bot. |
| ***DialogFlow*** | The dialog flow of the whole conversation and the nodes which it can go. |
| DialogDefinition | The developer can create their own nodes in the dialog tree, to let the developers create conversations to their needs. |
| ***Entity*** | An entity is the different options the system can prompt the user during a conversation. Entity is used to let the system know what steps to take the conversation forward. |
| **EntityDefinition** | Allows the developer to define their own entites. I.e. creating a new entity that is "I'm feeling good" for user questions like "How are you feeling?". |
| TrainingPhrases | Different user sentences matches one and the same intent. I.e. "What's the weather like?" and "How is the weather outside?" both being mapped to the intent: weather report. |
| NrOfIntents | The number of intents allowed within the system. |
| ***Intent*** | Intents are used to identify, what the user wants to know/ do using the system. |
| **IntentDefinition** | Allows the developer to define their own intents. I.e. creating a new intent that is "What time is it?" so that the system can understand the user if he/she asks for the time. |

| Continuation of Table 7 | |
|---|---|
| **Feature name** | **Description** |
| Synonyms | The system automatically takes into consideration to synonyms and phrases that have similar meaning. I.e. "large" and "extensive". |
| NrOfEntities | A restricted number of entities allowed within a system. |
| ***Speech*** | Features specific to speech and speech processing. |
| ToneAnalyzer | The system can analyse the tone of the user by using linguistic analysis to detect emotion and language tones. |
| VoiceActivityDetection | Voice activity detection is used for the system to understand when the user has stopped talking so that the system can shut off the microphone from listening any further. |
| | |
| ***InputModalities*** | The different input types supported by the system. |
| ImageInput | The system allows for image as an input, a image filetype such as .PNG, .JPEG, .TIFF, etc. |
| SpeechInput | The system allows for speech as an input, this means recordings of audio through a microphone. |
| TextInput | The system allows for text as an input, a string of characters that the user writes. |
| URLInput | The system allows for a URL as an input, an string that identifies to a websource on a network. This is used for redirection and lets the user choose webhook sources. |
| | |
| ***OutputModalities*** | The different output types supported by the system. |
| ImageOutput | The system has support to output an image as a response to an user request. |
| ListOutput | The system has support to output a list response to an user request, this list can contain options for the user to choose or simply a list of items that the user requested for. |
| TextOutput | The system has support to output a text as a response to an user request. |
| SpeechOutput | The system has support to output a text-to-speech response to an user request if the user has a speaker available. |
